# Supplementary material for: A Fast Learning-Based Surrogate of Electrical Machines using a Reduced Basis
Source: arXiv:2406.18990 source file (2024-06-27)
Supplement: Supplementary file 1 [file appendix2.tex]

\section{Appendix: a single-phase transformer }
\label{ap:use_case_single}

The single-phase transformer use case is composed of a cylinder and two windings. A winding is one or more turns of wire that form a continuous coil through which an electric current can pass. As can be seen in Figure \ref{use_case_1_section}, only one 2D section of this set is studied, thus the cylinder becomes a torus and the coils are represented by rectangles. The cylinder is made of metallic material with non-linear permeability. It is characterized by two Frolich coefficients: $\alpha= 0.00025$ and $\beta=0.00018$. The part of the domain not containing the cylinder contains air. The sections of the coils are represented by rectangles.
The electromagnetic problem (a primitive single-phase transformer) is magnetostatic. The wires of each coil are oriented as shown in Figure \ref{use_case_1_section}, a dot indicates that the current is circulating towards the reader. Each coil has a section equal to $50e-3 \cdot 100e-3$ m$^{2}=0.005$ m$^{2}$ and is composed of $1000$ turns. The boundary condition $B\cdot n = 0$ corresponding to a magnetic wall is imposed on all the boundaries of the domain. A magnetic vector potential type formulation A was used, and the numerical problems were solved by conjugate gradient and using a Jacobi pre-conditioner. The mesh of the use case shown in figure \ref{use_case_1_mesh} is irregular and composed of extruded triangles. It has 10,840 cells. The amplitude $A_1$ of the current $I_1$ is varied between $1$A and $20$A. The amplitude $A_2$ of the current $I_2$ is fixed at 0A. Current $I_1$ is imposed and is sinusoidal with frequency $f=50$Hz (
$I_1(t)= A_1\cdot\sin{(2\pi f t)}$, $I_2(t)= 0$). 
Each simulation is composed of $41$ time steps. Among all the information provided by the simulations, we are mainly interested in the magnetic field $B$ (this is one of the most interesting quantities) and more particularly in $B_x$, its component along the x-axis, for the sake of simplicity.

\begin{figure}[ht]
\centering
\begin{minipage}{.5\textwidth}
  \centering
  \begin{tikzpicture}[scale=1.6]
        \draw [fill=blue]  (0,0) circle (1) ;
        \draw [fill=white] (0,0) circle (0.85) ;
        \draw [->][dashed] (-1.8, -1.8) -- (-1.8, 1.8) node[left]{$y$} ;
        \draw [->][dashed] (-1.8, -1.8) -- (1.8, -1.8) node[below]{$x$} ;
        \draw (-1.8, -1.8) node[below left] {$z$};
        
        % Coil sections
        \draw (-1.4, -0.2) -- (-1.4, 0.2); 
        \draw (-1.4, 0.2) -- (-1.2, 0.2); 
        \draw (-1.2, 0.2) -- (-1.2, -0.2); 
        \draw (-1.2, -0.2) -- (-1.4, -0.2); 
        
        \draw (-0.6, -0.2) -- (-0.6, 0.2); 
        \draw (-0.6, 0.2) -- (-0.4, 0.2); 
        \draw (-0.4, 0.2) -- (-0.4, -0.2); 
        \draw (-0.4, -0.2) -- (-0.6, -0.2); 
        
        \draw (0.4, -0.2) -- (0.4, 0.2); 
        \draw (0.4, 0.2) -- (0.6, 0.2); 
        \draw (0.6, 0.2) -- (0.6, -0.2); 
        \draw (0.6, -0.2) -- (0.4, -0.2); 
        
        \draw (1.2, -0.2) -- (1.2, 0.2); 
        \draw (1.2, 0.2) -- (1.4, 0.2); 
        \draw (1.4, 0.2) -- (1.4, -0.2); 
        \draw (1.4, -0.2) -- (1.2, -0.2); 
        
        \draw[orange] (-1.3, 0) circle (0.08);
        \filldraw[orange] (-1.3,0) circle (0.5pt);
        \draw (1.3, 0) circle (0.08);
        \draw (-0.5, 0) circle (0.08);
        \filldraw[orange] (0.5,0) circle (0.5pt);
        \draw[orange] (0.5, 0) circle (0.08);
    
        \draw (-1.3,-0.2) node[below] {$I_1(t)$};
        \draw (0.5,-0.2) node[below] {$I_2(t)$};
        
        \draw (-0.5, 0.08) -- (-0.5, -0.08);
        \draw (1.3, 0.08) -- (1.3, -0.08);
    \end{tikzpicture}
  \caption{Geometry of the use case}
  \label{use_case_1_section}
\end{minipage}%
\begin{minipage}{.5\textwidth}
  \centering
  \includegraphics[width=.8\linewidth]{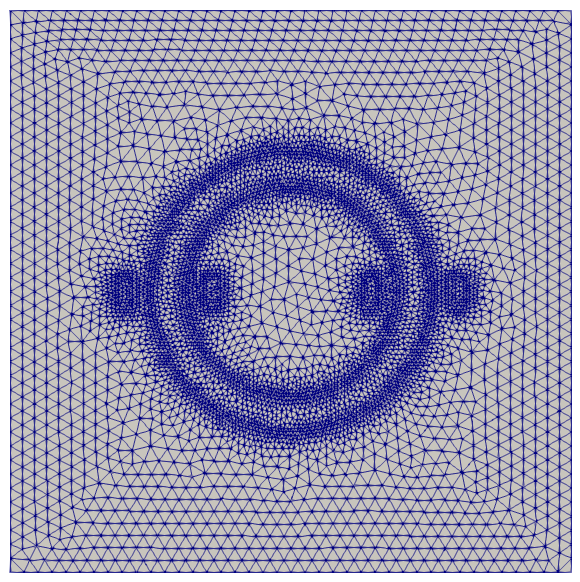}
  \caption{Mesh used in the simulations}
  \label{use_case_1_mesh}
\end{minipage}
\end{figure}
